# Supplementary material for: TEM Nanosculpting of Topological Insulator Bi$_2$Se$_3$
Source: arXiv:1712.02032 ancillary file (2017-12-06)
Supplement: Supplementary file 1 [file Supplementary_Information.pdf]

**Supplementary Figures**

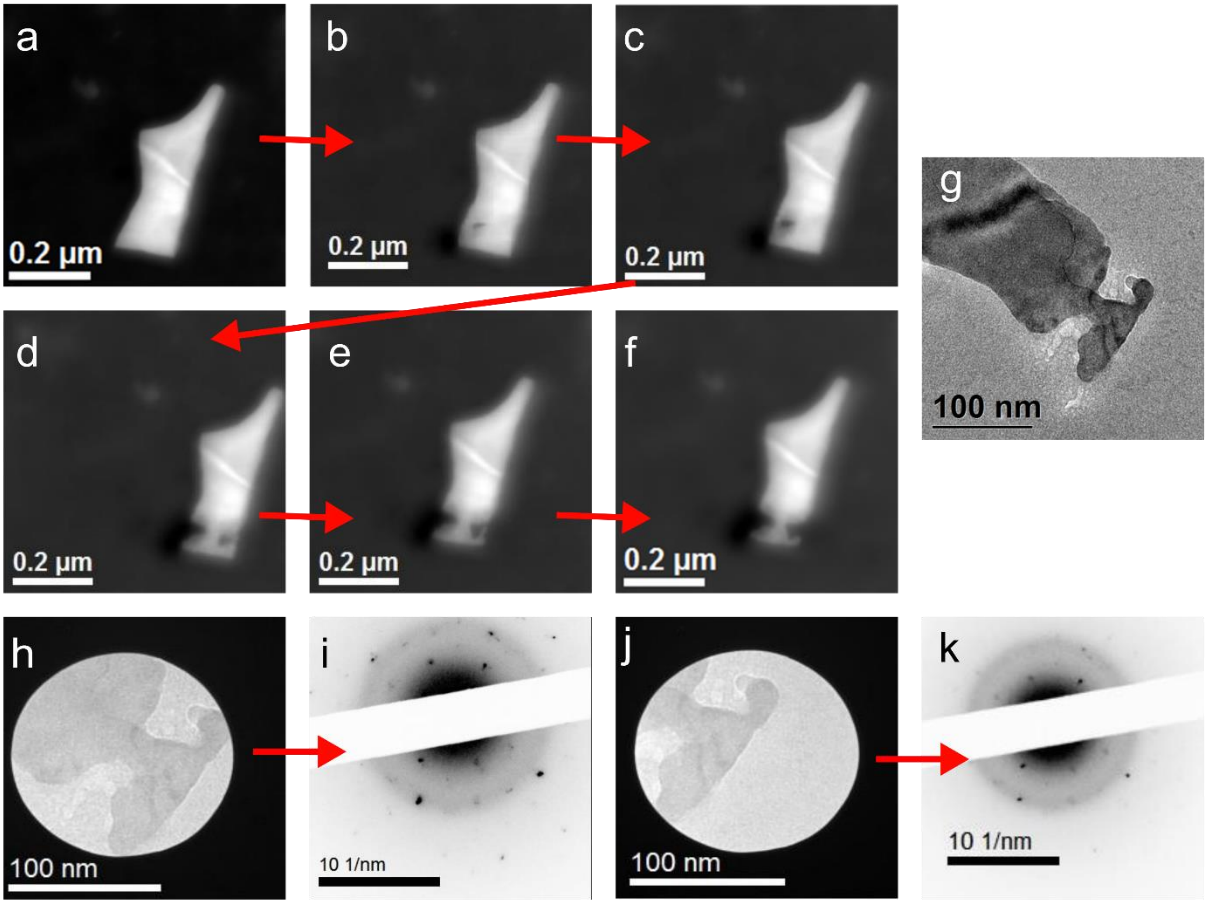


*Supplementary Figure S1: STEM images of another $Bi_2Se_3$ nanostructure as it is cut to create a small T-junction. In this trial, the beam current was increased to $4.8 \cdot 10^9\ A/m^2$ for cutting. a) before cutting b) 6 minutes of beam exposure c) 12 minutes of beam exposure d) 18 minutes of beam exposure e) 24 minutes of beam exposure f) 30 minutes of beam g) TEM image of final structure h-k) SAED of T-junction, showing the hexagonal symmetry of bismuth selenide. The diffraction pattern shows hexagonal symmetry, is aligned along the [001] zone axis, and has an average lattice spacing of 0.206 nm.*

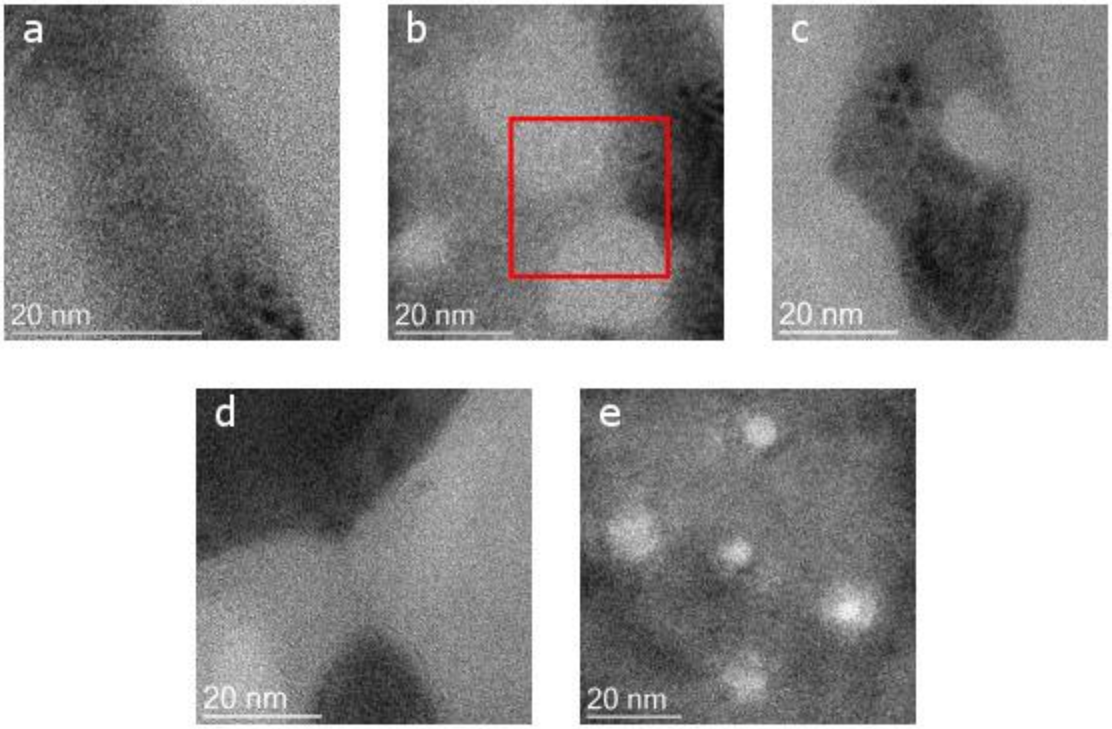


*Supplementary Figure S2: Grayscale image of TEM drilled structures (a) a 15 nm-wide wire (b) a thinner, shorter wire (c) a ring (d) a constriction (e) an antidot array.*

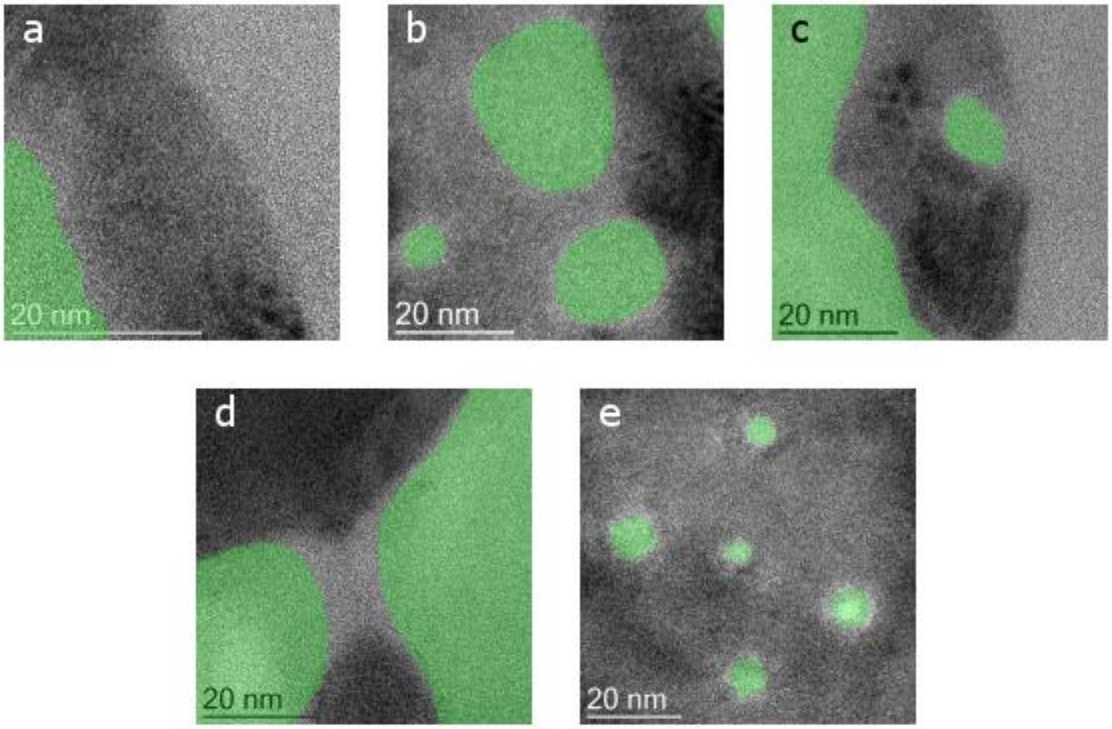


*Supplementary Figure S3: Gallery of drilled structures with spot-drilled areas highlighted in green.*

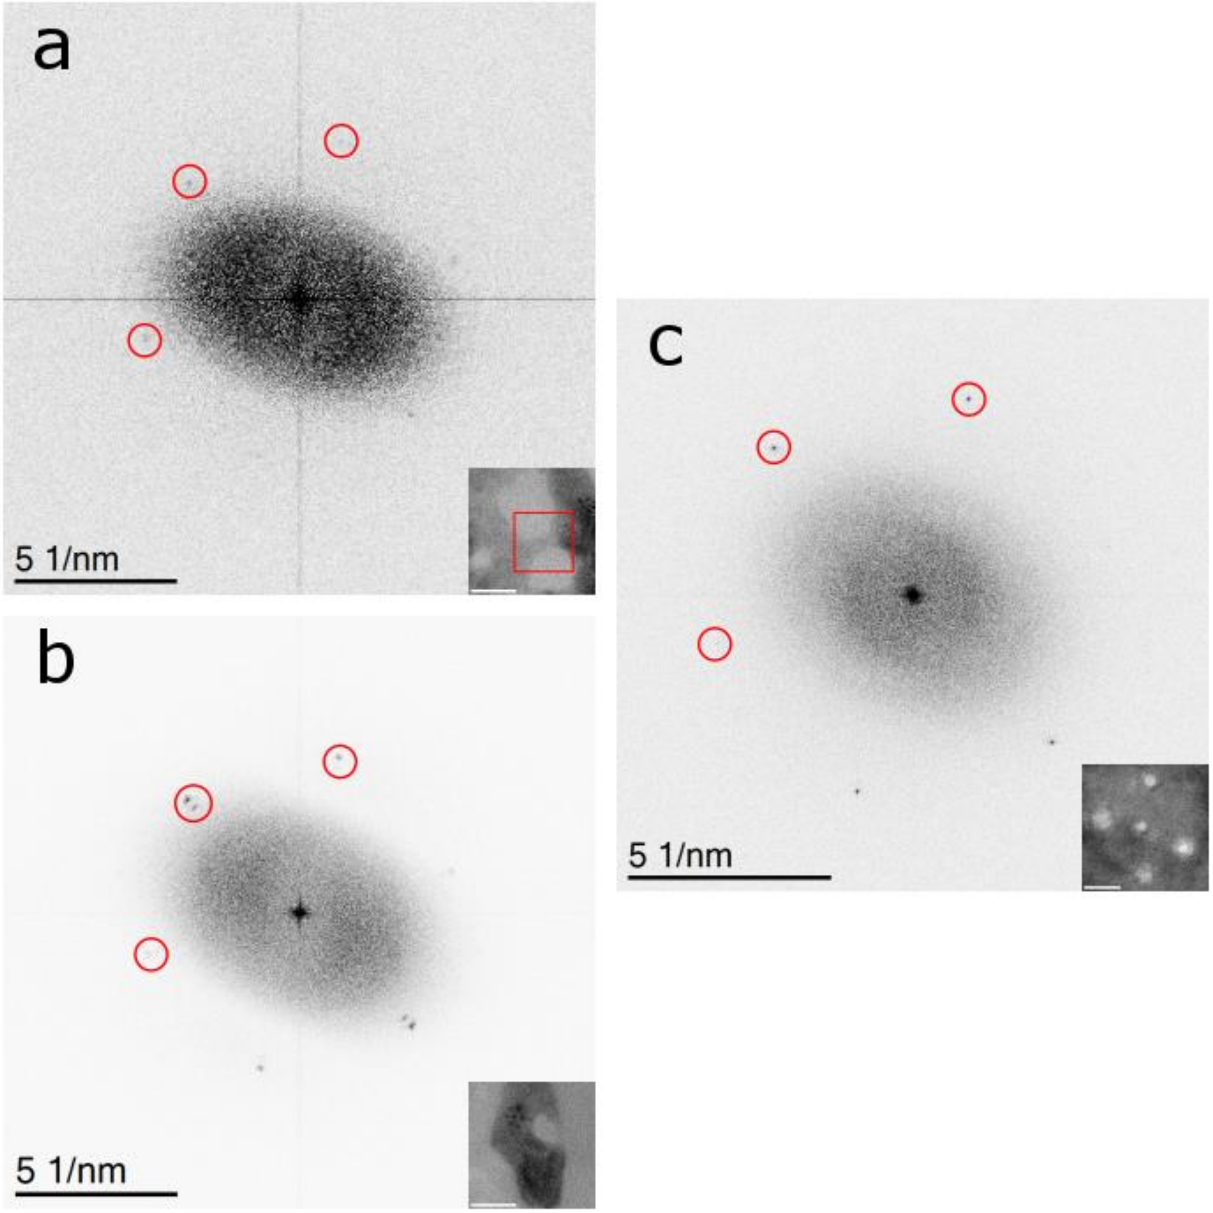


*Supplementary Figure S4: Selected enlarged FFTs from Figure 3, with selected areas inset.*

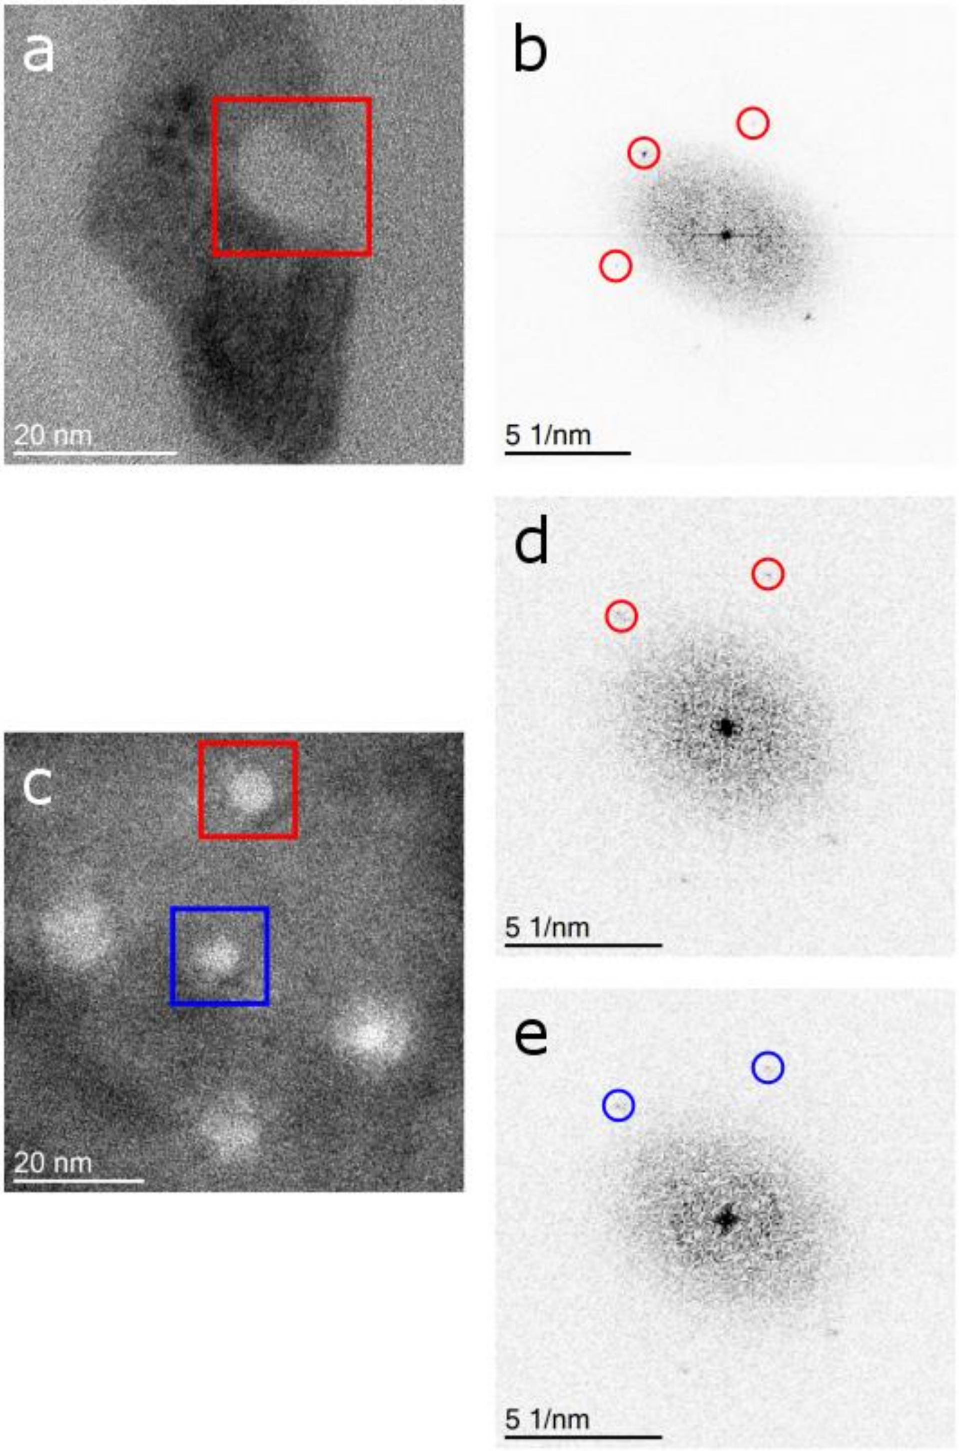


*Supplementary Figure S5: FFTs of exposed areas in the ring and antidot structures. a) Ring structure, with region selected for further analysis boxed in red. b) FFT of red boxed region in a) showing preservation of $Bi_2Se_3$ lattice spots. c) Antidot lattice with regions of interest boxed in red and blue. d) FFT of red boxed region in c), again showing presence of $Bi_2Se_3$ lattice spots. e) FFT of blue boxed region in c), showing much the same as d). In all FFTs, the spots are quite faint due to the smaller size of the ROI and due to the lower proportion of the ROI taken up by the bismuth selenide nanostructures.*

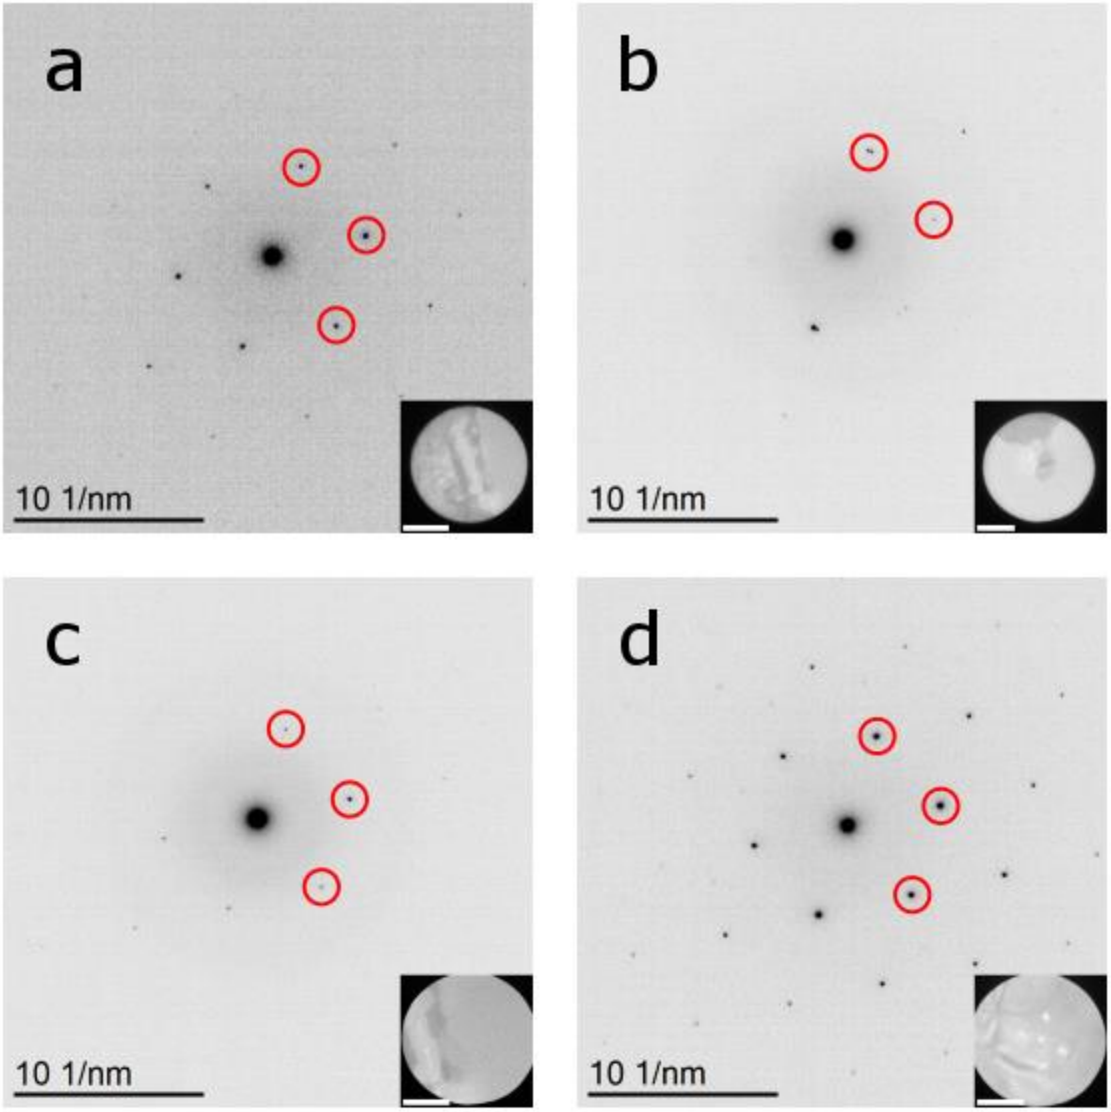


*Supplementary Figure S6 SAED of TEM-drilled structures with selected areas inset. Except where indicated, inset scale bars are 50 nm (a) Wire (b) Wire, ring, and adjacent structures (inset scale bar 100 nm (c) Constriction (d) Antidot lattice*

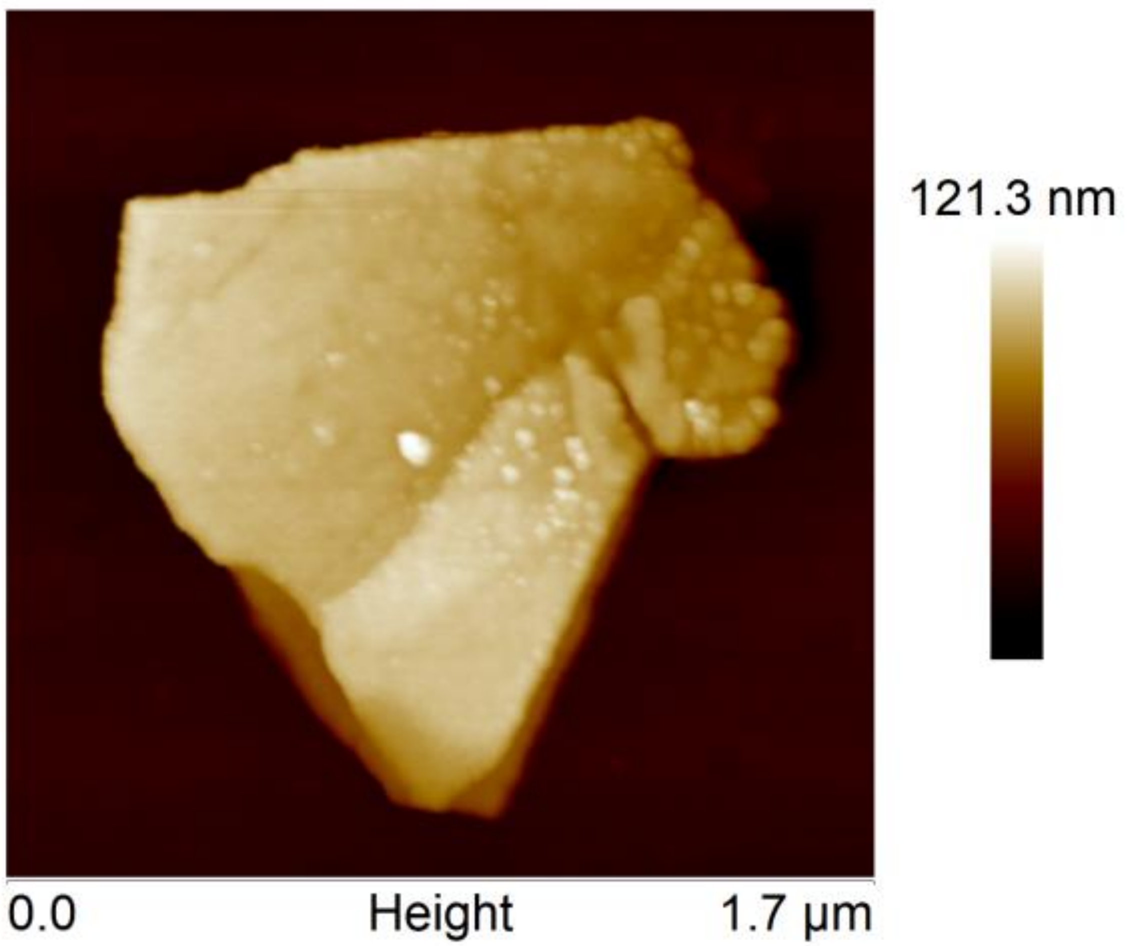


*Supplementary Figure S7: AFM image of thinned flake.*

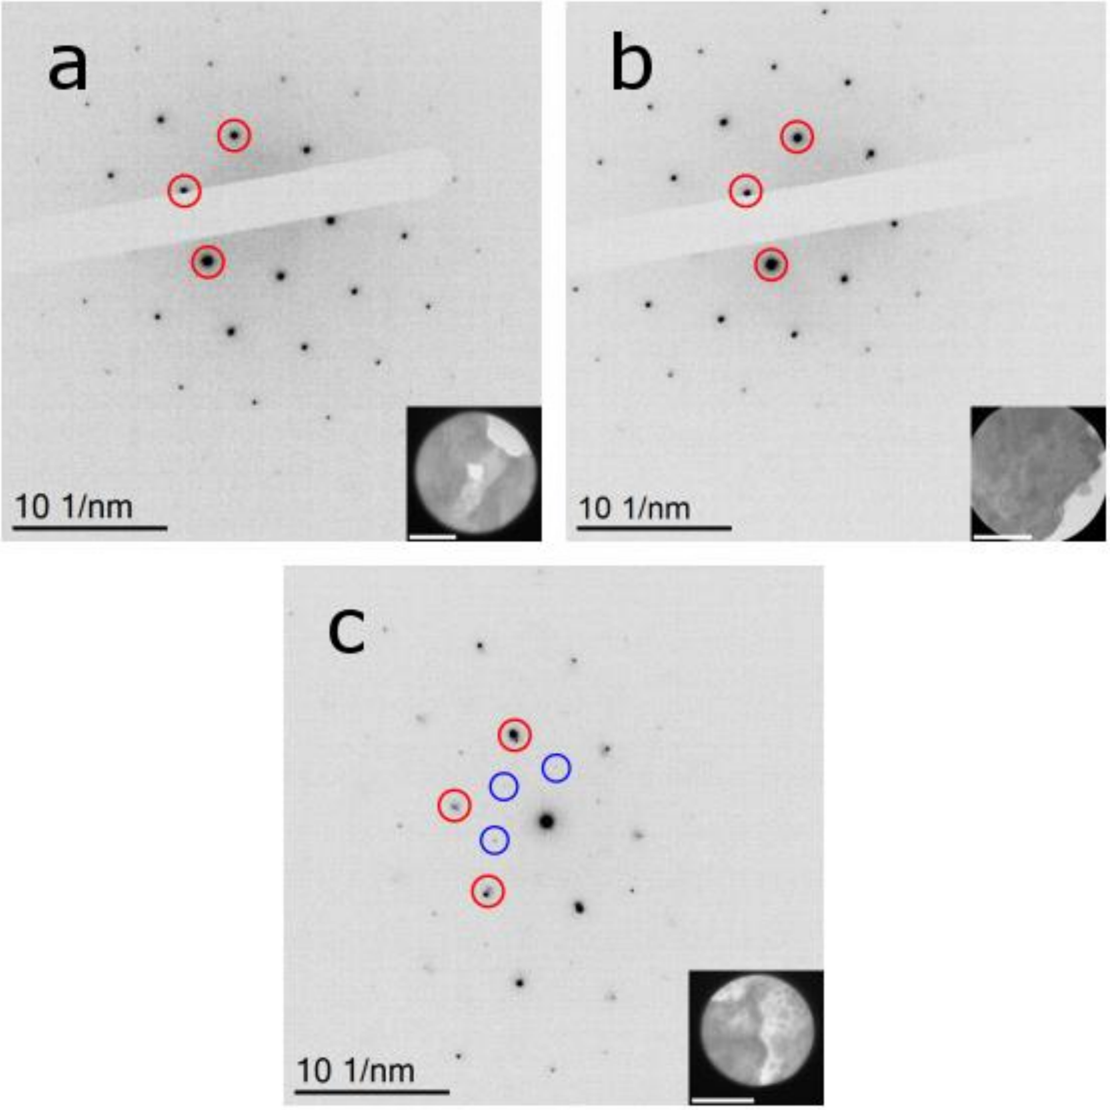


*Supplementary Figure S8 Selected-area diffraction of STEM-thinned samples with selected area inset (a) SAED of region shown in Figure 5(d). Average lattice spacing is 0.21 nm, consistent with bismuth selenide. (b) SAED of green boxed region shown in Figure 5(b). Average lattice spacing is 0.21 nm. (c) SAED of face-up thinned sample, showing two distinct hexagonal lattices. Representative points for each are circled in red and blue. The red-circled points correspond to an average lattice spacing of 0.17 nm, and the faint blue-circled points correspond to an average lattice spacing of 0.28 nm. In all insets, the scale bar is 100 nm.*

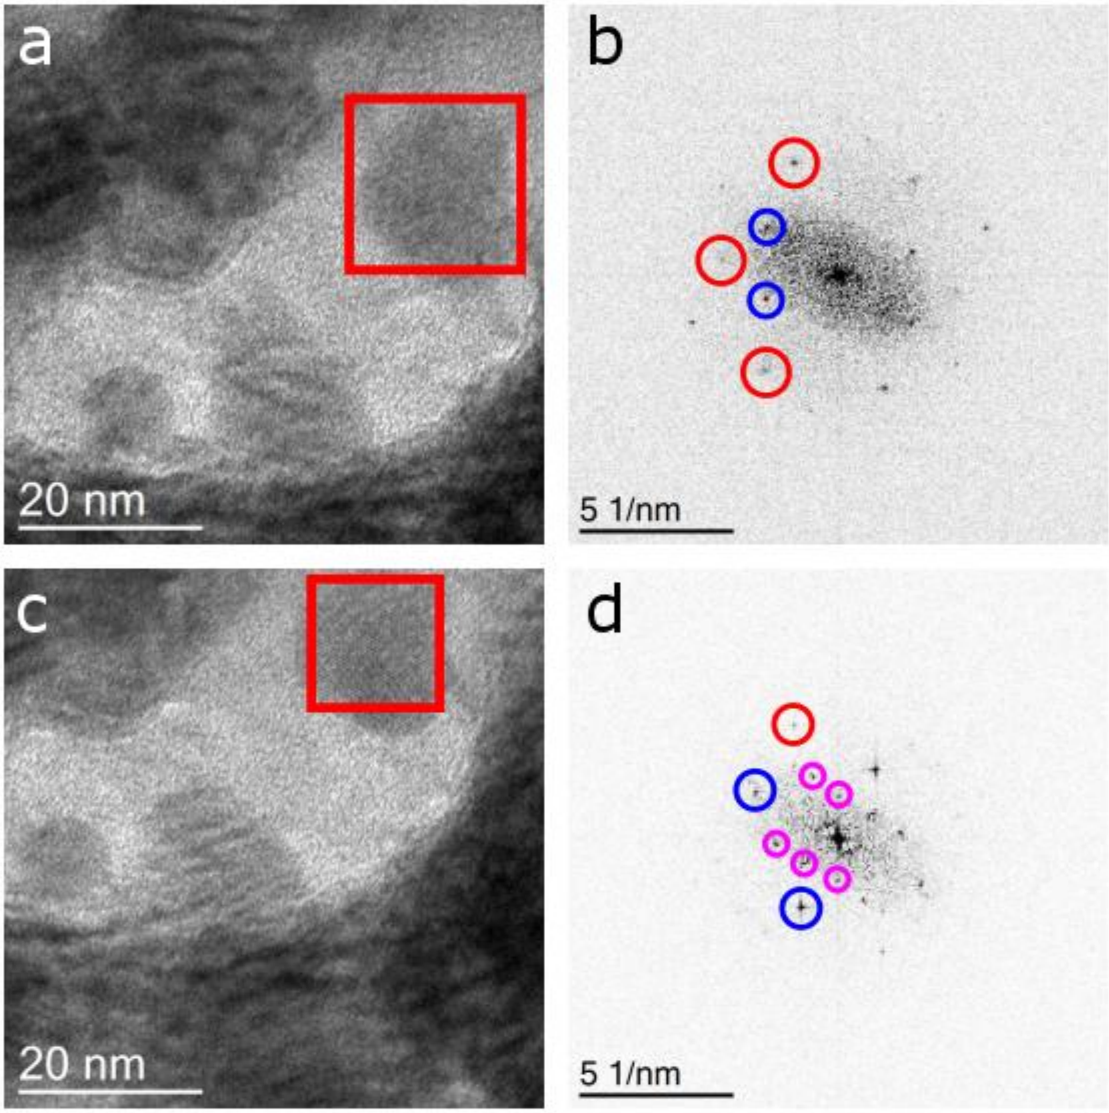


*Supplementary Figure S9: HRTEM and FFT of irradiated structures showing unusual imaging behavior. In a), the area outlined in red shows the typical lattice planes associated with the redeposited structures. Its FFT in b) shows the spots associated with these lattice planes circled in blue and the spots associated with $Bi_2Se_3$ lattice planes circled in red. The image shown in c), taken moments later, shows the same structure with unusual lattice fringes somewhat resembling masonry. Its FFT in d) shows radically different lattice planes, circled in magenta, although the blue-circled spots located at about 7:00 and 11:00 correspond to those shown in b). The red-circled dot corresponds to $Bi_2Se_3$ lattice spacing.*
